# Supplementary material for: Reading charge transport from spin dynamics on the surface of topological insulator
Source: arXiv:1303.4478 source file (2013-09-30)
Supplement: Supplementary file 1 [file appendix.pdf]

# Supplementary on-line material for "Reading charge transport from spin on the surface of topological insulator"

Xin Liu[1,2] and Jairo Sinova[1,3]

[1] *Department of Physics, Texas A&M University, College Station, TX 77843-4242, USA*
[2] *Department of Physics, The Pennsylvania State University, University Park, PA 16802-6300, USA*
[3] *Institute of Physics ASCR, Cukrovarnická 10, 162 53 Praha 6, Czech Republic*

(Dated: June 16, 2013)

In this appendix, we present the detailed calculation of the spin dynamics on the surface of topological insulator(TI) and how the spin polarization is constructed by the non-equilibrium electrons.

## SPIN-CHARGE DYNAMIC EQUATION

We assume that the low energy topological surface state(TSS) has the Dirac-like Hamiltonian plus nonmagnetic short range disorder potential [1, 2]

$$\hat{H} = v(\boldsymbol{z} \times \boldsymbol{\sigma}) \cdot \mathbf{k} + V_0 \Sigma_i \delta(\boldsymbol{r} - \boldsymbol{r}_i)\sigma_0, \tag{1}$$

where $v$ is the constant velocity, $\boldsymbol{z}$ is the unit vector perpendicular to the surface of TI, $\boldsymbol{k}$ is the wave vector of the electron, and $\sigma_0$ is $2 \times 2$ identical matrix. Here we assume $\hbar = 1$ and consider only the spin independent scattering. The velocity operator of this type of Hamiltonian has the form

$$\hat{\boldsymbol{V}} = \frac{\partial \hat{H}}{\partial \boldsymbol{k}} = v\boldsymbol{z} \times \boldsymbol{\sigma}, \tag{2}$$

and is proportional to the in plane spin polarization perpendicular to the velocity direction.

The dynamics of the spin-charge polarization, as a non-equilibrium process, can be naturally described by quantum kinetic equation [3]

$$\begin{aligned}&\partial_t \hat{G}^K + \nabla_{\mathbf{R}} \cdot [\frac{1}{2}\{\hat{\mathbf{V}}_k, \hat{G}^K\}] + i[\hat{H}_0(\boldsymbol{k}), \hat{G}^K] \\ &= -i\left[(\hat{\Sigma}^R \hat{G}^K - \hat{G}^K \hat{\Sigma}^A) - (\hat{G}^R \hat{\Sigma}^K - \hat{\Sigma}^K G^A)\right],\end{aligned} \tag{3}$$

where $t$ and $\boldsymbol{R}$ are time and real space variants, $\hat{G}^K$ is the $2\times2$ matrix of spin-$\frac{1}{2}$ Keldysh Green's function, $\hat{V} = v(\boldsymbol{z}\times\boldsymbol{\sigma})$ is the velocity operator, $\hat{H}_0(\boldsymbol{k}) = v(\boldsymbol{z} \times \boldsymbol{\sigma}) \cdot \boldsymbol{k}$ and $\Sigma^{R(A,K)}$ is the retarded (advanced,Keldysh) self energy due to disorder potential. The term $[\frac{1}{2}\{\hat{\mathbf{V}}_{\boldsymbol{k}}, G^K\}] = \hat{J}$ is natural definition of current matrix. The third term in the Eq. (3) is the spin torque exerted by the Rashba SOI. In this work, the operator with a hat means it is a matrix. In the equilibrium state, the Keldysh Green's function satisfies [3]

$$\hat{G}_0^K = (\hat{G}^R - \hat{G}^A)\tanh(\frac{E - \epsilon_f}{2k_B T}), \tag{4}$$

where $G_0^K$ stands Keldysh Green's function in equilibrium, $k_B$ is the Boltzmann constant and $T$ here is the system temperature. Based on Eq. (4) and we assume that the Keldysh Green's function generally has the form

$$\hat{G}^K = -2\pi i \delta(E - \epsilon_k^+)\hat{h}^+ - 2\pi i \delta(E - \epsilon_k^-)\hat{h}^-, \tag{5}$$

where $\epsilon_k^\pm = \pm vk$, $\hat{h}^\pm(\boldsymbol{k}, \boldsymbol{R}, T)$ is the distribution function, defined as

$$\hat{h}(\boldsymbol{k}, \boldsymbol{R}, t) = -\int_{-\infty}^{\infty} \frac{dE}{2\pi i} \hat{G}^K_{\boldsymbol{k},E}(\boldsymbol{R}, t) \tag{6}$$

and $\pm$ label the distribution function of the electrons spin sub-band above(below) Dirac point. Normally the non-equilibrium distribution function $\delta\hat{h}$ locate around Fermi energy. Therefore we define the non-equilibrium thermal average distribution function as

$$\hat{g}^\pm(\boldsymbol{e_k}, \boldsymbol{R}, t) = \int N(\epsilon_k) d\epsilon_k \delta\hat{h}^\pm(\boldsymbol{k}, \boldsymbol{R}, T) \tag{7}$$

where $\boldsymbol{e_k} = \boldsymbol{k}/k$ is the unit vector along $\boldsymbol{k}$ direction and $N(\epsilon_k) = k/hv$ is the density of state. In this work, we consider the case that the Fermi energy is above the Dirac point and much larger than $k_B T$.

To obtain the kinetic equation of distribution function, we introduce the non-equilibrium density matrix [4]

$$\hat{\rho}(R, t) = \frac{i}{2\pi N(\epsilon_k)} \int \frac{d^2k}{(2\pi)^2} \delta\hat{h} = \int \frac{d\theta}{2\pi} \delta\hat{g}(\boldsymbol{k_f}, \mathrm{R}, \mathrm{t}), \tag{8}$$

where $\theta$ is the angel between $\boldsymbol{k_f}$ and $x$ axis. By integrating out energy $E$ and $\epsilon_k$ The Eq. 3 can be converted to

$$\partial_t \hat{g} + \boldsymbol{\nabla}_{\boldsymbol{R}} \cdot \{\frac{1}{2}\hat{\boldsymbol{V}}, \hat{g}\} + i[\hat{H}(\boldsymbol{k_f}), \hat{g}] + \frac{\hat{g}}{\tau_p} = \frac{\hat{\rho}(\boldsymbol{R}, T)}{\tau_p}. \tag{9}$$

where

$$1/\tau_p = \frac{\pi n_i V_0^2}{\hbar} N(\epsilon_{k_f})$$

is the momentum scattering time at Fermi surface and $n_i$ is the 2D density of the nonmagnetic impurities.

The non-equilibrium thermal average distribution function and density matrix can be generally written as

$$\begin{aligned} \hat{g} &= g_c\sigma_0 + g_x\sigma_x + g_y\sigma_y + g_z\sigma_z, \\ \hat{\rho} &= \rho_c\sigma_0 + \rho_x\sigma_x + \rho_y\sigma_y + \rho_z\sigma_z. \end{aligned} \tag{10}$$

If we multiply $\sigma_i$ where $i = 0, x, y, z$ on both sides of Eq. 3 and calculate the trace, using the fact that $\mathrm{Tr}(\sigma_\mathrm{i}\sigma_\mathrm{j})/2 = \delta_\mathrm{ij}$, the quantum kinetic equation can be written in the classical spin-charge 4D space after integrating out $E$ as [4]

$$\hat{K} \begin{pmatrix} g_0 \\ g_x \\ g_y \\ g_z \end{pmatrix} = i \begin{pmatrix} \rho_0 \\ \rho_x \\ \rho_y \\ \rho_z \end{pmatrix}, \tag{11}$$

where

$$\hat{K} = \begin{pmatrix} \tilde{\Omega} & -i\tilde{\Delta}_y & i\tilde{\Delta}_x & 0 \\ -i\tilde{\Delta}_y & \tilde{\Omega} & 0 & -\tilde{\Omega}_{so}\cos(\theta) \\ i\tilde{\Delta}_x & 0 & \tilde{\Omega} & -\tilde{\Omega}_{so}\sin(\theta) \\ 0 & \tilde{\Omega}_{so}\cos(\theta) & \tilde{\Omega}_{so}\sin(\theta) & \tilde{\Omega} \end{pmatrix}, \tag{12}$$

$\tilde{\Omega} = 1 - i\omega\tau_p$, $\tilde{\Omega}_{so} = 2vk_f\tau_p$ and $\tilde{\Delta}_{x(y)} = lq_{x(y)}$ is from the anti-commutator on the left hand side of Eq. (9) which gives the spin-charge coupling. Here we have Fourier transformed $\partial_t$ and $\partial_{x(y)}$ to $-i\omega$ and $iq_{x(y)}$ which are the frequency and wavelength of the spin polarized wave. For convenience, in the rest of this paper we will express frequency in units of $1/\tau_p$ and wave vector in units of $1/l$, unless otherwise stated. The difficulty of obtaining the spin dynamics equation in the strong SOC regime lies on the fact that the three terms, spin precession angle $2vk_f\tau_p$, the dimensionless time and spacial spin relaxation rate $\omega\tau_p$ and $ql$, may be large simultaneously and cannot be treated perturbatively. Here, we abandon the idea of gradient expansion in terms of $\omega\tau_p$ and $ql$ and derive the spin-charge diffusion equation by simply multiplying $K^{-1}$ on both sides of Eq. (11) and integrating out the angle $\theta$. To simplify our discussion, we consider the spin wave vector is only along $x$ direction and takes $q_y = 0$. In this case, using the relation Eq. (11) the spin-charge dynamic equation of the density coefficient $\rho_{c(x,y,z)}$ can be obtained as

$$-i\int \frac{d\theta}{2\pi} \begin{pmatrix} g_0 \\ g_x \\ g_y \\ g_z \end{pmatrix} = \begin{pmatrix} \rho_0 \\ \rho_x \\ \rho_y \\ \rho_z \end{pmatrix} = \hat{D} \begin{pmatrix} \rho_0 \\ \rho_x \\ \rho_y \\ \rho_z \end{pmatrix}, \tag{13}$$

where $\hat{D} = \int \frac{d\theta}{2\pi}\hat{K}^{-1}$ and $\hat{K}^{-1}$ takes the form

$$\frac{\begin{pmatrix} \tilde{\Omega}\left(\tilde{\Omega}^2 + \tilde{\Omega}_{\mathrm{so}}^2\right) & i\cos(\theta)\sin(\theta)\tilde{\Delta}_x\tilde{\Omega}_{\mathrm{so}}^2 & -i\tilde{\Delta}_x\left(\tilde{\Omega}^2 + \cos^2(\theta)\tilde{\Omega}_{\mathrm{so}}^2\right) & -i\tilde{\Omega}\sin(\theta)\tilde{\Delta}_x\tilde{\Omega}_{\mathrm{so}} \\ i\cos(\theta)\sin(\theta)\tilde{\Delta}_x\tilde{\Omega}_{\mathrm{so}}^2 & \tilde{\Omega}\left(\tilde{\Omega}^2 + \tilde{\Delta}_x^2 + \sin^2(\theta)\tilde{\Omega}_{\mathrm{so}}^2\right) & -\tilde{\Omega}\cos(\theta)\sin(\theta)\tilde{\Omega}_{\mathrm{so}}^2 & \cos(\theta)\left(\tilde{\Omega}^2 + \tilde{\Delta}_x^2\right)\tilde{\Omega}_{\mathrm{so}} \\ -i\tilde{\Delta}_x\left(\tilde{\Omega}^2 + \cos^2(\theta)\tilde{\Omega}_{\mathrm{so}}^2\right) & -\tilde{\Omega}\cos(\theta)\sin(\theta)\tilde{\Omega}_{\mathrm{so}}^2 & \tilde{\Omega}^3 + \cos^2(\theta)\tilde{\Omega}_{\mathrm{so}}^2\tilde{\Omega} & \tilde{\Omega}^2\sin(\theta)\tilde{\Omega}_{\mathrm{so}} \\ i\tilde{\Omega}\sin(\theta)\tilde{\Delta}_x\tilde{\Omega}_{\mathrm{so}} & -\cos(\theta)\left(\tilde{\Omega}^2 + \tilde{\Delta}_x^2\right)\tilde{\Omega}_{\mathrm{so}} & -\tilde{\Omega}^2\sin(\theta)\tilde{\Omega}_{\mathrm{so}} & \tilde{\Omega}\left(\tilde{\Omega}^2 + \tilde{\Delta}_x^2\right) \end{pmatrix}}{\left(\tilde{\Omega}^2 + \tilde{\Omega}_{\mathrm{so}}^2\right)\tilde{\Omega}^2 + \tilde{\Delta}_x^2\left(\tilde{\Omega}^2 + \cos^2(\theta)\tilde{\Omega}_{\mathrm{so}}^2\right)} \tag{14}$$

The Eq. (13) is a generalized spin diffusion equation and valid from the weak to the strong SOC regime. It is noted that the denominator of $K^{-1}$ is the function of $\cos^2(\theta)$. By using the property of trigonometric functions without calculating the integral of $\theta$, it can be easily proved that the spin polarization along $x$ and $z$ direction is not coupled to other components. Therefore the Eq. (13) can be block diagonalized as

$$\begin{pmatrix} 1 - \frac{\tilde{\Omega}\left(\tilde{\Omega}^2+\tilde{\Omega}_{\mathrm{so}}^2\right)}{\tilde{\Omega}\sqrt{\tilde{\Omega}^2+\tilde{\Delta}_x^2}\sqrt{\tilde{\Omega}^2+\tilde{\Omega}_{\mathrm{so}}^2}\sqrt{\tilde{\Omega}^2+\tilde{\Delta}_x^2+\tilde{\Omega}_{\mathrm{so}}^2}} & i\left(\frac{1}{\tilde{\Delta}_x} - \frac{\tilde{\Omega}\sqrt{\tilde{\Omega}^2+\tilde{\Omega}_{\mathrm{so}}^2}}{\tilde{\Delta}_x\sqrt{\tilde{\Omega}^2+\tilde{\Delta}_x^2}\sqrt{\tilde{\Omega}^2+\tilde{\Delta}_x^2+\tilde{\Omega}_{\mathrm{so}}^2}}\right) \\ i\left(\frac{1}{\tilde{\Delta}_x} - \frac{\tilde{\Omega}\sqrt{\tilde{\Omega}^2+\tilde{\Omega}_{\mathrm{so}}^2}}{\tilde{\Delta}_x\sqrt{\tilde{\Omega}^2+\tilde{\Delta}_x^2}\sqrt{\tilde{\Omega}^2+\tilde{\Delta}_x^2+\tilde{\Omega}_{\mathrm{so}}^2}}\right) & 1 - \tilde{\Omega}\left(\frac{1}{\tilde{\Delta}_x^2} - \frac{\tilde{\Omega}\sqrt{\tilde{\Omega}^2+\tilde{\Omega}_{\mathrm{so}}^2}}{\tilde{\Delta}_x^2\sqrt{\tilde{\Omega}^2+\tilde{\Delta}_x^2}\sqrt{\tilde{\Omega}^2+\tilde{\Delta}_x^2+\tilde{\Omega}_{\mathrm{so}}^2}}\right) \end{pmatrix} \begin{pmatrix} \rho_0 \\ \rho_y \end{pmatrix} = 0 \tag{15}$$

$$\begin{pmatrix} 1-(\frac{\sqrt{\tilde{\Omega}^2+\tilde{\Delta}_x^2}\sqrt{\tilde{\Omega}^2+\tilde{\Delta}_x^2+\tilde{\Omega}_{\rm so}^2}}{\tilde{\Delta}_x^2\sqrt{\tilde{\Omega}^2+\tilde{\Omega}_{\rm so}^2}}-\frac{\tilde{\Omega}}{\tilde{\Delta}_x^2}) & 0 \\ 0 & 1-\frac{\sqrt{\tilde{\Omega}^2+\tilde{\Delta}_x^2}}{\sqrt{\tilde{\Omega}^2+\tilde{\Omega}_{\rm so}^2}\sqrt{\tilde{\Omega}^2+\tilde{\Delta}_x^2+\tilde{\Omega}_{\rm so}^2}} \end{pmatrix} \begin{pmatrix} \rho_x \\ \rho_z \end{pmatrix} = 0 \tag{16}$$

For the spin-charged coupled equation, Eq. 15, when the spin is uniformly polarized, say $\tilde{\Delta}_x = 0$, the off diagonal terms in the spin dynamic matrix vanish. Therefore, the charge and spin densities for the uniform polarization are independent.

## IN-PLANE SPIN DYNAMICS UNDER DIFFUSIVE APPROXIMATION

In this section, we derive the spin dynamics equation under the diffusive approximation, $|\omega|\tau_p \ll 1$ and $ql \ll 1$ and show our method gives the same results to the spin dynamic equation in Ref.5 obtained from the Kubo formula. We focus on the in-plane spin polarization along $x$ direction. It has been proved exactly to not couple the spin polarization in other directions. Therefore we only need to calculate the element $\hat{D}_{22}$ which takes the form

$$\hat{D}_{22} = \int \frac{d\theta}{2\pi} \frac{-\sin^2\theta\cos\theta\tilde{\Delta}_x\tilde{\Omega}_{\rm so}^2 + \tilde{\Omega}\left(\tilde{\Omega}^2+\tilde{\Delta}_x^2+\sin^2(\theta)\tilde{\Omega}_{\rm so}^2\right)}{\left(\tilde{\Omega}^2+\tilde{\Omega}_{\rm so}^2\right)\tilde{\Omega}^2+\tilde{\Delta}_x^2\left(\tilde{\Omega}^2+\cos^2(\theta)\tilde{\Omega}_{\rm so}^2\right)}, \tag{17}$$

Due to the fact that $\sin^2(\theta+\pi)\cos(\theta+\pi) = -\sin^2\theta\cos\theta$, we can drop the fist term in the integrated function of Eq. 17 and have

$$\hat{D}_{22} = \int \frac{d\theta}{2\pi} \frac{\tilde{\Omega}\left(\tilde{\Omega}^2+\tilde{\Delta}_x^2+\sin^2(\theta)\tilde{\Omega}_{\rm so}^2\right)}{\left(\tilde{\Omega}^2+\tilde{\Omega}_{\rm so}^2\right)\tilde{\Omega}^2+\tilde{\Delta}_x^2\left(\tilde{\Omega}^2+\cos^2(\theta)\tilde{\Omega}_{\rm so}^2\right)}. \tag{18}$$

Taking the diffusive approximation $\tilde{\Delta}_x \ll 1$ and $\omega\tau_p \ll 1$ while $\tilde{\Omega}_{so} \gg 1$, we expand the Eq. 18 up to the first nonzero order in terms of $\tilde{\Delta}_x$ and $\tilde{\Omega}_{so}$ as

$$\begin{aligned} \hat{D}_{22} &= \int \frac{d\theta}{2\pi} \frac{\tilde{\Omega}\left(\tilde{\Omega}^2+\tilde{\Delta}_x^2+\sin^2(\theta)\tilde{\Omega}_{\rm so}^2\right)}{\left(\tilde{\Omega}^2+\tilde{\Omega}_{\rm so}^2\right)\tilde{\Omega}^2+\tilde{\Delta}_x^2\left(\tilde{\Omega}^2+\cos^2(\theta)\tilde{\Omega}_{\rm so}^2\right)} \\ &\approx \int \frac{d\theta}{2\pi} \frac{\tilde{\Omega}\sin^2\theta}{\tilde{\Omega}^2+\tilde{\Delta}_x^2\cos^2\theta} \\ &\approx \int \frac{d\theta}{2\pi} \frac{(1-i\omega\tau_p)\sin^2\theta}{1-2i\omega\tau_p+\tilde{\Delta}_x^2\cos^2\theta} \\ &\approx \int \frac{d\theta}{2\pi} \left((1-i\omega\tau_p)\sin^2\theta + 2i\omega\tau_p\sin^2\theta + \tilde{\Delta}_x^2\cos^2\theta\sin^2\theta\right) \\ &\approx \int \frac{d\theta}{2\pi} \left((1+i\omega\tau_p)\frac{1-\cos 2\theta}{2} + \tilde{\Delta}_x^2\frac{1-\cos 4\theta}{8}\right) \approx \frac{1}{2}(1+i\omega\tau_p-\frac{\tilde{\Delta}_x^2}{4}). \end{aligned} \tag{19}$$

Substituting Eq. 19 to the generalized spin dynamic equation Eq. 13, we have

$$i\omega\tau_p = 1 + \frac{1}{4}\tilde{\Delta}_x^2, \tag{20}$$

which can be Fourier transformed to the real space as

$$\partial_t\rho_x = -\frac{1}{2}D_s\partial_x^2\rho_x - \frac{\rho_x}{\tau_p}, \tag{21}$$

where $D_s = v_f^2\tau_p/2$. This is equivalent to the in-plane spin diffusive equation in Ref.5. (Here we assuming spin wave vector along x direction and the term contain $\partial_y$ is zero).

## THE SPIN POLARIZATION TEXTURE IN 2DEG AND ON THE SURFACE OF TI

In this section, we intuitively show why spin helix mode is absent on the surface of TI. In the following derivation, we focus on the $k_y = 0$ channel to simple our calculation.

The spin wave operator in real space is defined as

$$\hat{S}_+(x) = \sum_k \left( C^\dagger_{k+q,\uparrow} C_{k,\downarrow} \frac{e^{-iqx}}{2} \begin{pmatrix} 1 & -i \\ -i & -1 \end{pmatrix} + C^\dagger_{k,\downarrow} C_{k+q,\uparrow} \frac{e^{iqx}}{2} \begin{pmatrix} 1 & i \\ i & -1 \end{pmatrix} \right) \tag{22}$$

and

$$\hat{S}_-(x) = \sum_k \left( C^\dagger_{k-q,\uparrow} C_{k,\downarrow} \frac{e^{iqx}}{2} \begin{pmatrix} 1 & -i \\ -i & -1 \end{pmatrix} + C^\dagger_{k,\downarrow} C_{k-q,\uparrow} \frac{e^{-iqx}}{2} \begin{pmatrix} 1 & i \\ i & -1 \end{pmatrix} \right) \tag{23}$$

First, let us consider the spin polarization on the 2DEG. The operator $\hat{S}_+$ actin on electron states gets an spin density wave which has the form

$$\begin{aligned} S_+(x) = \hat{S}_+|\psi\rangle &= \sum_k \left( \sqrt{h_{k,\downarrow}(1-h_{k+q,\uparrow})} \frac{e^{-iqx}}{2} \begin{pmatrix} 1 & -i \\ -i & -1 \end{pmatrix} \right) \\ &+ \sum_k \left( \sqrt{h_{k+q,\uparrow}(1-h_{k,\downarrow})} \frac{e^{iqx}}{2} \begin{pmatrix} 1 & i \\ i & -1 \end{pmatrix} \right) \\ &= \sum_k \sqrt{h_k(1-h_k)} \left( \cos(qx)\sigma_z - \sin(qx)\sigma_x \right). \end{aligned} \tag{24}$$

where $h_{k,\uparrow(\downarrow)}$ is occupied probability which is the diagonal element of the distribution function in Eq. 6. Here, in the case of $q \ll k_f$, we make an approximation that $h_{k+q,\uparrow} = h_{k,\downarrow}$. The spin polarization given by Eq. 24 in three directions are $\langle S_z \rangle = \cos(qx)$, $\langle S_x \rangle = -\sin(qx)$ and $\langle S_y \rangle$=0 which is a contour-clock wise spin helix mode in $x - z$ plane.

Similar the clockwise spin helix mode is constructed by

$$\begin{aligned} S_- = \langle \hat{S}_-(x) \rangle &= \sum_k \left( \sqrt{f_{k-q,\uparrow} f_{k,\downarrow} (1-f_{k-q,\uparrow})(1-fk,\downarrow)} \frac{e^{iqx}}{2} \begin{pmatrix} 1 & -i \\ -i & -1 \end{pmatrix} \right) \\ &+ \sum_k \left( \sqrt{f_{k-q,\uparrow} f_{k,\downarrow} (1-f_{k-q,\uparrow})(1-fk,\downarrow)} \frac{e^{-iqx}}{2} \begin{pmatrix} 1 & i \\ i & -1 \end{pmatrix} \right) \\ &\approx \sum_k \sqrt{h_k(1-h_k)} \left( \cos(qx)\sigma_z + \sin(qx)\sigma_x \right), \end{aligned} \tag{25}$$

whose spin polarization in three directions are $\langle S_z \rangle = \cos(qx)$, $\langle S_x \rangle = \sin(qx)$ and $\langle S_y \rangle = 0$.

On the surface of TI, there is only one spin-sub band at the Fermi surface. The other sub-band is below the Dirac point and thereby far below the Fermi energy in the condition $E_f \gg kT$. Accordingly, for the counter-clockwise spin helix mode in Eq. 24, $h_{k+q,\uparrow}$ and $h_{k,\downarrow}$ can not be approximately equal because they belong to different spin-sub band and has the energy difference about $2E_f$. For example, when $k < 0$, as shown in Fig.1b in the paper, the state $|k+q,\uparrow\rangle$ is below the Dirac point and completely occupied so that $h_{k+q<0,\downarrow} = 1$. Similar we also have $h_{k>0,\uparrow} = 1$. As a result, the terms containing $\sum_{k>0} C^\dagger_{k,\downarrow} C_{k+q,\uparrow}$ ($\sum_{k+q<0} C^\dagger_{k+q,\uparrow} C_{k,\downarrow}$) becomes zero because they are proportional to $\sqrt{1-h_{k+q<0,\uparrow}} = 0$($\sqrt{1-h_{k>0,\downarrow}} = 0$). This implies hat only half terms in Eq. 24 which have the form

$$\begin{aligned} S_+^{\text{half}} &= \sum_{k+q>0} \langle C^\dagger_{k+q,\uparrow} C_{k,\downarrow} \rangle + \sum_{k<0} \langle C^\dagger_{k,\downarrow} C_{k+q,\uparrow} \rangle \\ &= \sum_{k+q>0} \sqrt{1-h_{k+q,\uparrow}} \frac{e^{-iqx}}{2} \begin{pmatrix} 1 & -i \\ -i & -1 \end{pmatrix} + \sum_{k<0} \sqrt{1-h_{k,\downarrow}} \frac{e^{iqx}}{2} \begin{pmatrix} 1 & i \\ i & -1 \end{pmatrix} \end{aligned} \tag{26}$$

will contribute to the spin polarization. Similar, for the clockwise spin helix mode, only half terms in Eq. 25 which have the form

$$\begin{aligned} S_-^{\text{half}} &= \sum_{k-q>0} \langle C^\dagger_{k-q,\uparrow} C_{k\downarrow} \rangle + \sum_{k<0} \langle C^\dagger_{k,\downarrow} C_{k-q,\uparrow} \rangle \\ &= \sum_{k-q>0} \sqrt{1-h_{k-q,\uparrow}} \frac{e^{iqx}}{2} \begin{pmatrix} 1 & -i \\ -i & -1 \end{pmatrix} + \sum_{k<0} \sqrt{1-h_{k,\downarrow}} \frac{e^{-iqx}}{2} \begin{pmatrix} 1 & i \\ i & -1 \end{pmatrix} \end{aligned} \tag{27}$$

will contribute to the spin polarization. By redefining $k+q \to k$ and $k-q \to k$ in Eq. 26 and Eq. 27 separately, we obtain the spin polarization on the surface as

$$\begin{aligned} S = S_{+}^{\mathrm{half}} + S_{-}^{\mathrm{half}} &= \sum_{k>0} \sqrt{1-h_{k,\uparrow}} \frac{e^{-iqx}}{2} \begin{pmatrix} 1 & -i \\ -i & -1 \end{pmatrix} + \sum_{k<0} \sqrt{1-h_{k,\downarrow}} \frac{e^{iqx}}{2} \begin{pmatrix} 1 & i \\ i & -1 \end{pmatrix} \\ &+ \sum_{k>0} \sqrt{1-h_{k,\uparrow}} \frac{e^{iqx}}{2} \begin{pmatrix} 1 & -i \\ -i & -1 \end{pmatrix} + \sum_{k<0} \sqrt{1-h_{k,\downarrow}} \frac{e^{-iqx}}{2} \begin{pmatrix} 1 & i \\ i & -1 \end{pmatrix} \\ &= \sum_{k>0} \sqrt{1-h_{k,\uparrow}} \cos(qx)\sigma_z + \sum_{k<0} \sqrt{1-h_{k,\downarrow}} \cos(qx)\sigma_z = \sum_{k} \sqrt{1-h_k^{+}} \cos(qx)\sigma_z, \end{aligned} \tag{28}$$

where $h_k^+$ is the distribution of the spin-sub band above Dirac point and defined in Eq. 5 and Eq. 6 which only has finite spin polarization along $z$ direction and will not couple to $x$ direction.


[1] M. Z. Hasan and C. L. Kane, Rev. Mod. Phys. **82**, 3045 (2010).
[2] X.-L. Qi and S.-C. Zhang, Rev. Mod. Phys. **83**, 1057 (2011).
[3] J. Rammer, Quantum Field Theory of Non-equilibrium States (Cambridge University Press, 2007).
[4] X. Liu and J. Sinova, Phys. Rev. B **86**, 174301 (2012).
[5] A. A. Burkov and D. G. Hawthorn, Phys. Rev. Lett. **105**, 066802 (2010).
